# Supplementary material for: Globally Resonant Homoclinic Tangencies
Source: arXiv:2206.08630 source file (2022-06-17)
Supplement: Supplementary file 1 [file appendix1.tex]

\chapter{A Typical Appendix...}

...consists of all the junk that you couldn't fit into the main part of the thesis, like more tables of data.
